# Supplementary material for: Asymmetric Non-local Neural Networks for Semantic Segmentation
Source: arXiv:1908.07678 source file (2019-08-29)
Supplement: Supplementary file 1 [file appendix_full.tex]

\documentclass[10pt,twocolumn,letterpaper]{article}

\usepackage{iccv}
\usepackage{times}
\usepackage{epsfig}
\usepackage{graphicx}
\usepackage{amsmath}
\usepackage{amssymb}
\usepackage{booktabs}

% Include other packages here, before hyperref.

% If you comment hyperref and then uncomment it, you should delete
% egpaper.aux before re-running latex.  (Or just hit 'q' on the first latex
% run, let it finish, and you should be clear).
\usepackage[pagebackref=true,breaklinks=true,letterpaper=true,colorlinks,bookmarks=false]{hyperref}

\usepackage[belowskip=-12pt,aboveskip=1pt]{caption}
\captionsetup{font={footnotesize}}

\iccvfinalcopy % *** Uncomment this line for the final submission

 % *** Enter the ICCV Paper ID here

% \newcommand{\zzhu}[1]{{\color{blue} ZZ: ``#1''}}

% Pages are numbered in submission mode, and unnumbered in camera-ready
% \ificcvfinal\pagestyle{empty}\fi
\begin{document}

%%%%%%%%% TITLE
	\title{Supplementary Materials for Asymmetric Non-local Neural Networks for Semantic Segmentation}
	
	\maketitle
	\input{latex/appendix.tex}
	
	{\small
	    \bibliographystyle{ieee_fullname}
		\bibliography{egbib}
	}
	
\end{document}
